# Supplementary material for: Exploring Latent Pathways: Enhancing the Interpretability of Autonomous Driving with a Variational Autoencoder
Source: arXiv:2404.01750 source file (2024-04-02)
Supplement: Supplementary file 1 [file automatic_latent_plot.tex]

The standard technique to interpret the information encoded in each latent dimension of VAE is to perform a latent perturbation analysis. This consists of taking the latent encoding of a given input, then to change the value of only one perturbation at the time and observe the change in the reconstructed image. For a small number of dimensions, the analysis can be carried out by an experienced human operator in a reasonable time. However in the  case of large number of dimensions, this operation becomes intractable for human. Additionally, a higher number of dimension means that the information is more diffused thus noticing the changes in the perturbated  reconstructions becomes highly difficult even for the eye of a trained expert, for example see \autoref{fig:dim0}

\begin{figure*}[!htb]
	\includegraphics[width=\textwidth]{material/dim0.png}
	\caption{Latent perturbation for latent dimension 0 (out of 256). The image in the center is the original input image. The images on the right and extreme-right represent respectively the perturbated reconstructions of the center image by adding respectively +1$\sigma$ and +$\sigma$ from the value of dimension 0. The images on the left and extreme-left represent respectively the perturbated reconstructions of the center image by subtracting respectively +1$\sigma$ and +$\sigma$ from the value of dimension 0. Here $\sigma$ represents the standard deviation of the distribution of the dimension 0.}
	\label{fig:dim0}
\end{figure*}

For this purpose, we developed an automatic assistant that indicates the detected changes and overlays them on top of the perturbated reconstruction. This simplifies the analysis task for the human operator and draws his attention to all possible differences between the extreme right and extreme left perturbated images as seen in \autoref{fig:alp0}.

\begin{figure}[!htb]
	\includegraphics[width=0.4\textwidth]{material/alp0.png}
	\caption{ALP plot for dimension 0. Top-center image represents the original input image. Top-right and top-left represent respectively the extreme-right and extreme-left images from \autoref{fig:dim0}. Bottom row images are each overlayed with the difference mask from \autoref{fig:diff0}, from left to right: extreme-left image, segmentation map of the (estimated using a DL model), extreme-right image.}
	\label{fig:alp0}
\end{figure}

\begin{figure}[!htb]
	\includegraphics[width=0.4\textwidth]{material/diff0.png}
	\caption{The difference image is obtained by subtracting the extreme-left image from the extreme-right one, then summing over the channels of its absolute value and finally thresholding over its normalization (by its maximum value) with the $90\textsuperscript{th}$ quantile as threshold.}
	\label{fig:diff0}
\end{figure}
