# Supplementary material for: Exploring Latent Pathways: Enhancing the Interpretability of Autonomous Driving with a Variational Autoencoder
Source: arXiv:2404.01750 source file (2024-04-02)
Supplement: Supplementary file 2 [file vae_archi.tex]

\begin{figure*}[h]
	\begin{verbatim}
Model: "encoder"
__________________________________________________________________________________________________
Layer (type)                   Output Shape         Param #     Connected to                     
==================================================================================================
input_layer (InputLayer)       [(None, 78, 200, 4)  0           []                               
							   ]                                                                 

conv_1 (Conv2D)                (None, 39, 100, 8)   296         ['input_layer[0][0]']            

bn_1 (BatchNormalization)      (None, 39, 100, 8)   32          ['conv_1[0][0]']                 

relu_1 (ReLU)                  (None, 39, 100, 8)   0           ['bn_1[0][0]']                   

conv_2 (Conv2D)                (None, 20, 50, 16)   1168        ['relu_1[0][0]']                 

bn_2 (BatchNormalization)      (None, 20, 50, 16)   64          ['conv_2[0][0]']                 

relu_2 (ReLU)                  (None, 20, 50, 16)   0           ['bn_2[0][0]']                   

conv_3 (Conv2D)                (None, 10, 25, 32)   4640        ['relu_2[0][0]']                 

bn_3 (BatchNormalization)      (None, 10, 25, 32)   128         ['conv_3[0][0]']                 

relu_3 (ReLU)                  (None, 10, 25, 32)   0           ['bn_3[0][0]']                   

conv_4 (Conv2D)                (None, 5, 13, 64)    18496       ['relu_3[0][0]']                 

bn_4 (BatchNormalization)      (None, 5, 13, 64)    256         ['conv_4[0][0]']                 

relu_4 (ReLU)                  (None, 5, 13, 64)    0           ['bn_4[0][0]']                   

flatten (Flatten)              (None, 4160)         0           ['relu_4[0][0]']                 

mean (Dense)                   (None, 32)           133152      ['flatten[0][0]']                

log_var (Dense)                (None, 32)           133152      ['flatten[0][0]']                

sampling (Sampling)            (None, 32)           0           ['mean[0][0]',                   
'log_var[0][0]']                

==================================================================================================
Total params: 291,384
Trainable params: 291,144
Non-trainable params: 240
	\end{verbatim}
	\caption{Convolutional \acrshort{vae} encoder architecture.}
	\label{fig:encoder}
\end{figure*}

\begin{figure*}[h!]
	\begin{verbatim}
Model: "Decoder"
_________________________________________________________________
Layer (type)                Output Shape              Param #   
=================================================================
input_layer (InputLayer)    [(None, 32)]              0         

dense_1 (Dense)             (None, 4160)              137280    

Reshape (Reshape)           (None, 5, 13, 64)         0         

conv_transpose_1 (Conv2DTra  (None, 10, 26, 64)       36928     
nspose)                                                         

bn_1 (BatchNormalization)   (None, 10, 26, 64)        256       

relu_1 (ReLU)               (None, 10, 26, 64)        0         

conv_transpose_2 (Conv2DTra  (None, 20, 52, 32)       18464     
nspose)                                                         

bn_2 (BatchNormalization)   (None, 20, 52, 32)        128       

relu_2 (ReLU)               (None, 20, 52, 32)        0         

conv_transpose_3 (Conv2DTra  (None, 40, 104, 16)      4624      
nspose)                                                         

bn_3 (BatchNormalization)   (None, 40, 104, 16)       64        

relu_3 (ReLU)               (None, 40, 104, 16)       0         

conv_transpose_4 (Conv2DTra  (None, 80, 208, 8)       1160      
nspose)                                                         

bn_4 (BatchNormalization)   (None, 80, 208, 8)        32        

relu_4 (ReLU)               (None, 80, 208, 8)        0         

conv_transpose_5 (Conv2DTra  (None, 80, 208, 4)       292       
nspose)                                                         

resizing (Resizing)         (None, 78, 200, 4)        0         

=================================================================
Total params: 199,228
Trainable params: 198,988
Non-trainable params: 240
	\end{verbatim}
	\caption{Convolutional \acrshort{vae} decoder architecture.}
	\label{fig:decoder}
\end{figure*}
