# Supplementary material for: Exploring Latent Pathways: Enhancing the Interpretability of Autonomous Driving with a Variational Autoencoder
Source: arXiv:2404.01750 source file (2024-04-02)
Supplement: Supplementary file 3 [file usecases.tex]

\begin{figure}[!htb]
	\includegraphics[width=0.4\textwidth]{material/usecase1.jpg}
	\label{fig:usecase1}
\end{figure}

\begin{figure}[!htb]
	\includegraphics[width=0.4\textwidth]{material/usecase2.jpg}
	\label{fig:usecase2}
\end{figure}

\begin{figure}[!htb]
	\includegraphics[width=0.4\textwidth]{material/usecase3.jpg}
	\label{fig:usecase3}
\end{figure}

\begin{figure}[!htb]
	\includegraphics[width=0.4\textwidth]{material/usecase4.jpg}
	\label{fig:usecase4}
\end{figure}
