# Supplementary material for: Exploring Latent Pathways: Enhancing the Interpretability of Autonomous Driving with a Variational Autoencoder
Source: arXiv:2404.01750 source file (2024-04-02)
Supplement: Supplementary file 4 [file vista.tex]

\textcolor{red}{[PLACE HOLDER] GIVE DETAILS ON VISTA ITSELF AND ON OUR CONTRIBUTIONS TO IT.}
